# Supplementary material for: Combining the $\Delta$-Self-Consistent-Field and GW Methods for Predicting Core Electron Binding Energies in Periodic Solids
Source: arXiv:2306.05928 ancillary file (2023-06-09)

Supplementary Information for

Combining the  $\Delta$ -Self-Consistent-Field and  
GW Methods for Predicting Core Electron  
Binding Energies in Periodic Solids

J. Matthias Kahk<sup>†</sup> and Johannes Lischner<sup>‡</sup>

*<sup>†</sup>Institute of Physics, University of Tartu, W. Ostwaldi 1, 50411 Tartu, Estonia  
email: juhan.matthias.kahk@ut.ee*

*<sup>‡</sup>Department of Physics and Department of Materials, and the Thomas Young Centre for Theory and  
Simulation of Materials, Imperial College London, London SW7 2AZ, United Kingdom*

# Table of Contents

|                                                                                               |    |
|-----------------------------------------------------------------------------------------------|----|
| Binding energies from Eqn. 1 and Eqn. 3, extrapolation.....                                   | 3  |
| BeO.....                                                                                      | 3  |
| Beryllium.....                                                                                | 4  |
| $\beta$ -SiC.....                                                                             | 5  |
| Diamond.....                                                                                  | 6  |
| Graphite.....                                                                                 | 7  |
| hex-BN.....                                                                                   | 8  |
| Lithium.....                                                                                  | 9  |
| Magnesium.....                                                                                | 10 |
| Silicon.....                                                                                  | 11 |
| Sodium.....                                                                                   | 12 |
| Numerical verification of Eqn. 2.....                                                         | 13 |
| Structures and k-point grids used in the GW and GW $\Gamma$ calculations.....                 | 15 |
| BeO.....                                                                                      | 15 |
| Be metal.....                                                                                 | 15 |
| $\beta$ -SiC.....                                                                             | 15 |
| Diamond.....                                                                                  | 15 |
| Graphite.....                                                                                 | 16 |
| hex-BN.....                                                                                   | 16 |
| Li metal.....                                                                                 | 16 |
| Mg metal.....                                                                                 | 16 |
| Silicon.....                                                                                  | 17 |
| Na metal.....                                                                                 | 17 |
| Extrapolation of the GW and GW $\Gamma$ results to $E_{\text{cut}} \Rightarrow +\infty$ ..... | 18 |
| BeO.....                                                                                      | 18 |
| Be metal.....                                                                                 | 18 |
| $\beta$ -SiC.....                                                                             | 19 |
| Diamond.....                                                                                  | 19 |
| Graphite.....                                                                                 | 20 |
| hex-BN.....                                                                                   | 20 |
| Li metal.....                                                                                 | 21 |
| Mg metal.....                                                                                 | 21 |
| Silicon.....                                                                                  | 22 |
| Na metal.....                                                                                 | 22 |

# Binding energies from Eqn. 1 and Eqn. 3, extrapolation

## BeO

| Supercell | Atoms per supercell | (Atoms per supercell) <sup>(-1/3)</sup> | O 1s B.E.,<br>Eqn. 1, PBE | O 1s B.E.,<br>Eqn. 3, PBE | Be 1s B.E.,<br>Eqn. 1, PBE | Be 1s B.E.,<br>Eqn. 3, PBE |
|-----------|---------------------|-----------------------------------------|---------------------------|---------------------------|----------------------------|----------------------------|
| 1x1x1     | 4                   | 0.630                                   | 525.75                    | 526.66                    | 107.82                     | 108.74                     |
| 2x2x1     | 16                  | 0.397                                   | 526.56                    | 526.91                    | 108.80                     | 109.14                     |
| 3x3x2     | 72                  | 0.240                                   | 527.24                    | 527.39                    | 109.48                     | 109.62                     |
| 4x4x3     | 196                 | 0.172                                   | 527.52                    | 527.62                    | 109.76                     | 109.86                     |
| 5x5x3     | 300                 | 0.149                                   | 527.60                    | 527.68                    | 109.84                     | 109.93                     |
| 6x6x3     | 432                 | 0.132                                   | 527.67                    | 527.75                    | 109.92                     | 109.99                     |

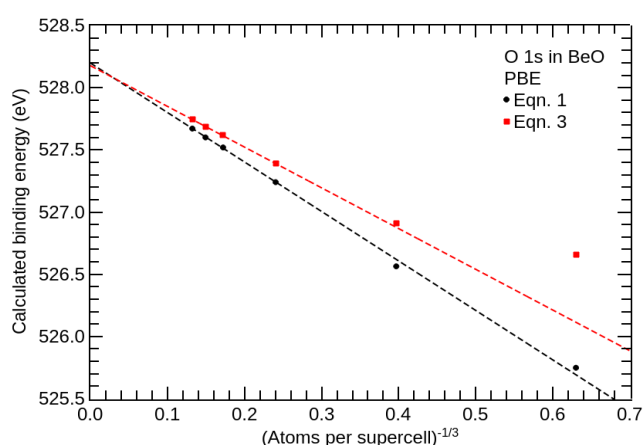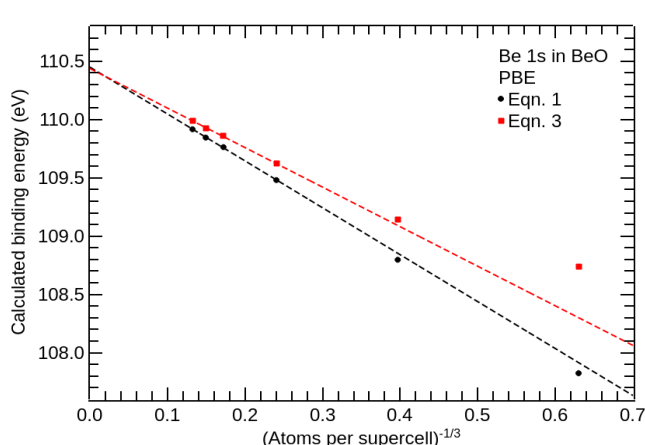

| Supercell | Atoms per supercell | (Atoms per supercell) <sup>(-1/3)</sup> | O 1s B.E.,<br>Eqn. 1, SCAN | O 1s B.E.,<br>Eqn. 3, SCAN | Be 1s B.E.,<br>Eqn. 1, SCAN | Be 1s B.E.,<br>Eqn. 3, SCAN |
|-----------|---------------------|-----------------------------------------|----------------------------|----------------------------|-----------------------------|-----------------------------|
| 1x1x1     | 4                   | 0.630                                   | 526.34                     | 527.26                     | 108.07                      | 108.98                      |
| 2x2x1     | 16                  | 0.397                                   | 527.16                     | 527.50                     | 109.06                      | 109.41                      |
| 3x3x2     | 72                  | 0.240                                   | 527.85                     | 528.01                     | 109.77                      | 109.91                      |
| 4x4x3     | 196                 | 0.172                                   | 528.15                     | 528.25                     | 110.07                      | 110.17                      |
| 5x5x3     | 300                 | 0.149                                   | 528.23                     | 528.32                     | 110.16                      | 110.24                      |
| 6x6x3     | 432                 | 0.132                                   | 528.31                     | 528.38                     | 110.23                      | 110.31                      |

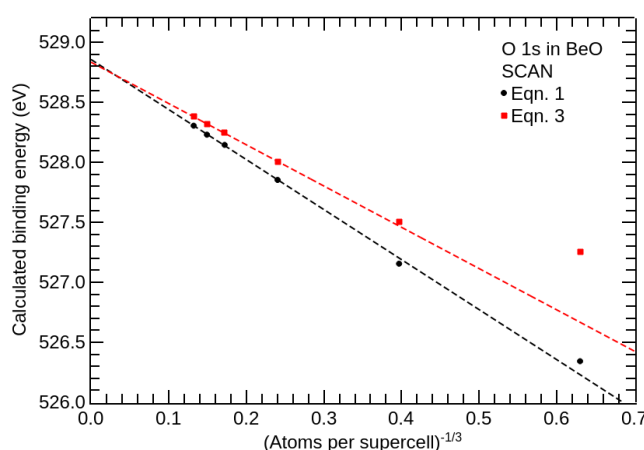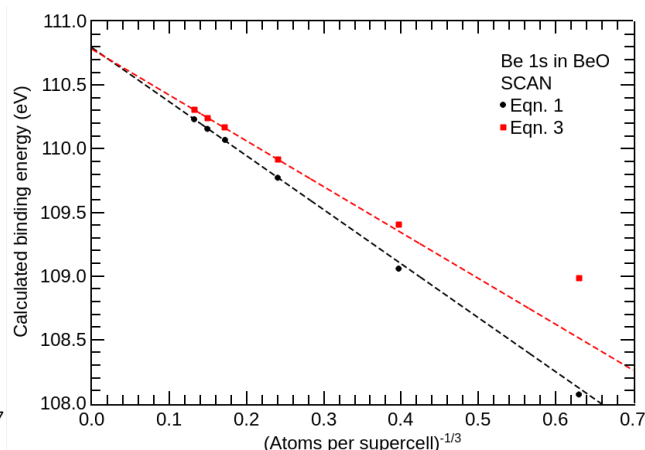

# Beryllium

| Supercell | Atoms per<br>supercell | (Atoms per<br>supercell) <sup>-1/3</sup> | Be 1s B.E.,<br>Eqn. 1, PBE | Be 1s B.E.,<br>Eqn. 3, PBE | Be 1s B.E.,<br>Eqn. 1, SCAN | Be 1s B.E.,<br>Eqn. 3, SCAN |
|-----------|------------------------|------------------------------------------|----------------------------|----------------------------|-----------------------------|-----------------------------|
| 1x1x1     | 2                      | 0.794                                    | 109.89                     | 111.24                     | 110.24                      | 112.04                      |
| 2x2x1     | 8                      | 0.500                                    | 110.70                     | 111.29                     | 111.07                      | 111.69                      |
| 3x3x2     | 36                     | 0.303                                    | 111.24                     | 111.38                     | 111.66                      | 111.81                      |
| 4x4x3     | 96                     | 0.218                                    | 111.37                     | 111.43                     | 111.80                      | 111.87                      |
| 5x5x3     | 150                    | 0.188                                    | 111.44                     | 111.51                     | 111.89                      | 111.95                      |
| 6x6x4     | 288                    | 0.151                                    | 111.43                     | 111.45                     | 111.87                      | 111.91                      |

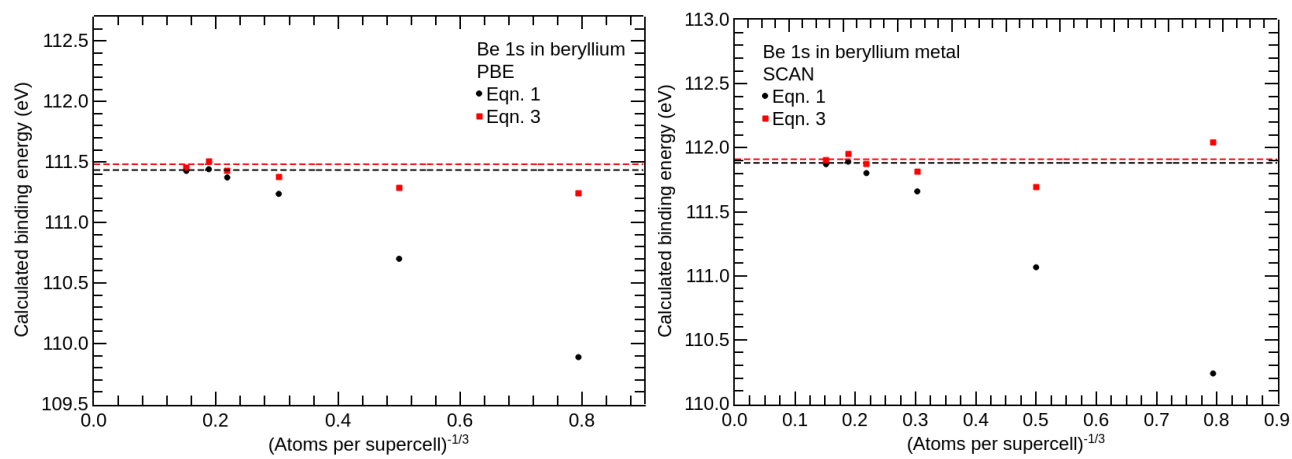

## $\beta$ -SiC

| Supercell | Atoms per<br>supercell | (Atoms per<br>supercell) <sup>(-1/3)</sup> | C 1s B.E.,<br>Eqn. 1, PBE | C 1s B.E.,<br>Eqn. 3, PBE | Si 2p B.E.,<br>Eqn. 1, PBE | Si 2p B.E.,<br>Eqn. 3, PBE |
|-----------|------------------------|--------------------------------------------|---------------------------|---------------------------|----------------------------|----------------------------|
| 1x1x1     | 2                      | 0.794                                      | 279.22                    | 280.40                    | 96.82                      | 98.00                      |
| 2x2x2     | 16                     | 0.397                                      | 280.32                    | 280.64                    | 98.22                      | 98.53                      |
| 3x3x3     | 54                     | 0.265                                      | 280.52                    | 280.55                    | 98.34                      | 98.48                      |
| 4x4x4     | 128                    | 0.198                                      | 280.62                    | 280.72                    | 98.44                      | 98.54                      |
| 5x5x5     | 250                    | 0.159                                      | 280.68                    | 280.76                    | 98.51                      | 98.58                      |

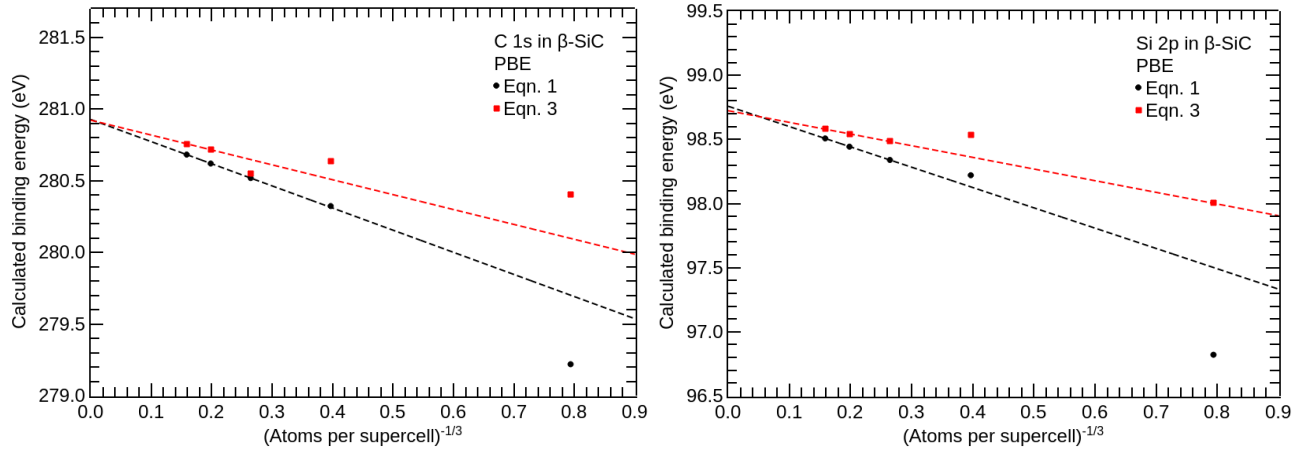

| Supercell | Atoms per<br>supercell | (Atoms per<br>supercell) <sup>(-1/3)</sup> | C 1s B.E.,<br>Eqn. 1, SCAN | C 1s B.E.,<br>Eqn. 3, SCAN | Si 2p B.E.,<br>Eqn. 1, SCAN | Si 2p B.E.,<br>Eqn. 3, SCAN |
|-----------|------------------------|--------------------------------------------|----------------------------|----------------------------|-----------------------------|-----------------------------|
| 1x1x1     | 2                      | 0.794                                      | 279.68                     | 280.88                     | 98.42                       | 99.62                       |
| 2x2x2     | 16                     | 0.397                                      | 280.82                     | 281.14                     | 98.50                       | 98.82                       |
| 3x3x3     | 54                     | 0.265                                      | 281.04                     | 281.19                     | 98.76                       | 98.91                       |
| 4x4x4     | 128                    | 0.198                                      | 281.15                     | 281.25                     | 98.88                       | 98.97                       |
| 5x5x5     | 250                    | 0.159                                      | 281.22                     | 281.29                     | 98.95                       | 99.02                       |

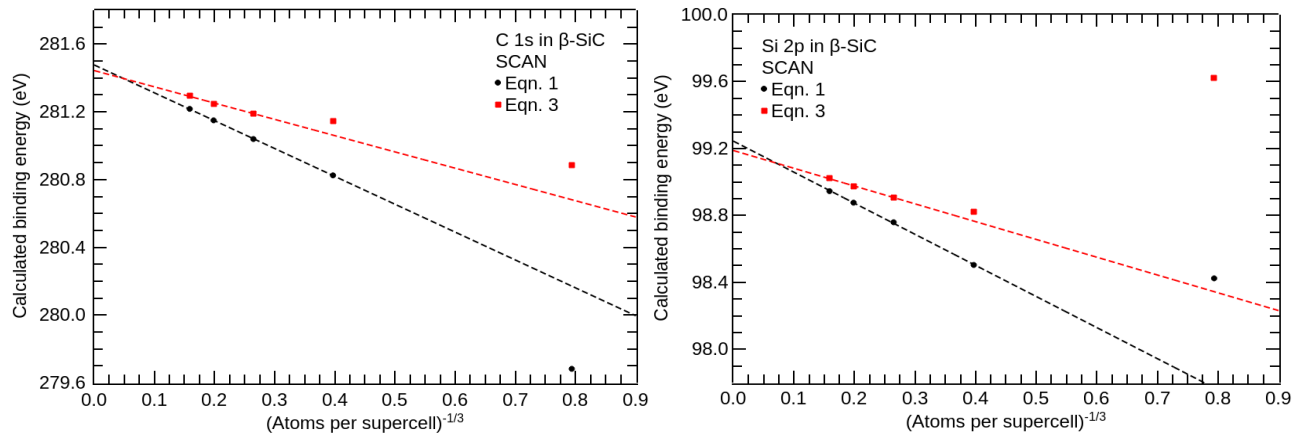

# Diamond

| Supercell | Atoms per<br>supercell | (Atoms per<br>supercell) <sup>-1/3</sup> | C 1s B.E.,<br>Eqn. 1, PBE | C 1s B.E.,<br>Eqn. 3, PBE | C 1s B.E.,<br>Eqn. 1, SCAN | C 1s B.E.,<br>Eqn. 3, SCAN |
|-----------|------------------------|------------------------------------------|---------------------------|---------------------------|----------------------------|----------------------------|
| 1x1x1     | 2                      | 0.794                                    | 280.34                    | 282.86                    | 280.93                     | 283.48                     |
| 2x2x2     | 16                     | 0.397                                    | 282.55                    | 283.33                    | 283.11                     | 283.91                     |
| 3x3x3     | 54                     | 0.265                                    | 283.07                    | 283.44                    | 283.66                     | 283.99                     |
| 4x4x4     | 128                    | 0.198                                    | 283.31                    | 283.52                    | 283.81                     | 284.09                     |
| 5x5x5     | 250                    | 0.159                                    | 283.45                    | 283.59                    | 284.00                     | 284.15                     |
| 6x6x6     | 432                    | 0.132                                    | 283.51                    | 283.62                    | 284.05                     | 284.17                     |

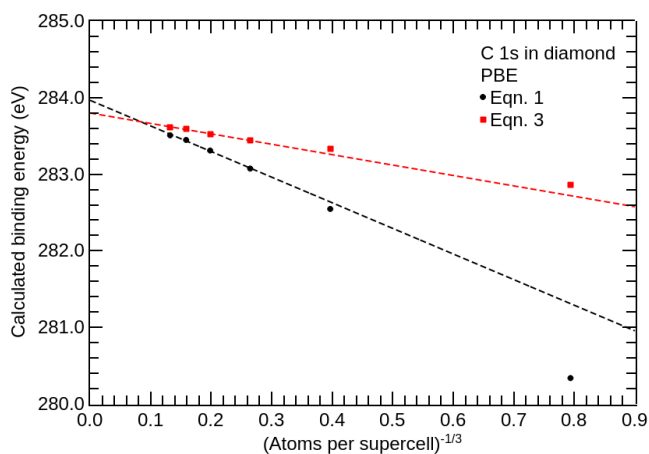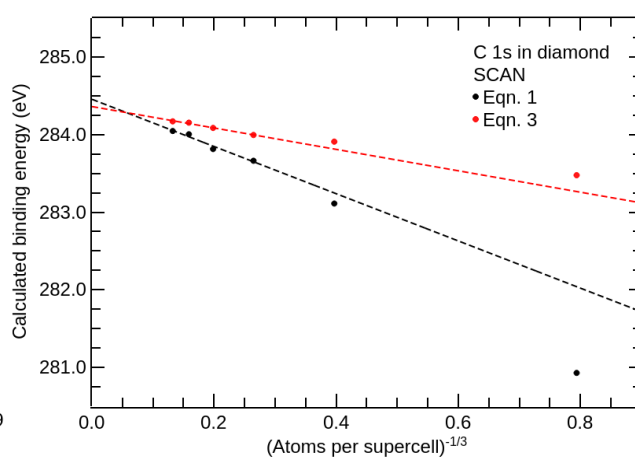

# Graphite

| Supercell | Atoms per<br>supercell | (Atoms per<br>supercell) <sup>-1/3</sup> | C 1s B.E.,<br>Eqn. 1, PBE | C 1s B.E.,<br>Eqn. 3, PBE | C 1s B.E.,<br>Eqn. 1, SCAN | C 1s B.E.,<br>Eqn. 3, SCAN |
|-----------|------------------------|------------------------------------------|---------------------------|---------------------------|----------------------------|----------------------------|
| 1x1x1     | 4                      | 0.630                                    | 282.39                    | 284.26                    | 283.26                     | 285.11                     |
| 2x2x2     | 32                     | 0.315                                    | 283.10                    | 283.78                    | 283.92                     | 284.61                     |
| 3x3x3     | 108                    | 0.210                                    | 283.28                    | 283.62                    | 284.09                     | 284.44                     |
| 4x4x4     | 256                    | 0.157                                    | 283.37                    | 283.56                    | 284.18                     | 284.38                     |
| 2x2x1     | 16                     | 0.397                                    | 282.48                    | 283.45                    | 283.24                     | 284.22                     |
| 4x4x2     | 128                    | 0.198                                    | 283.14                    | 283.45                    | 283.95                     | 284.26                     |
| 6x6x3     | 432                    | 0.132                                    | 283.30                    | 283.45                    | 284.11                     | 284.26                     |

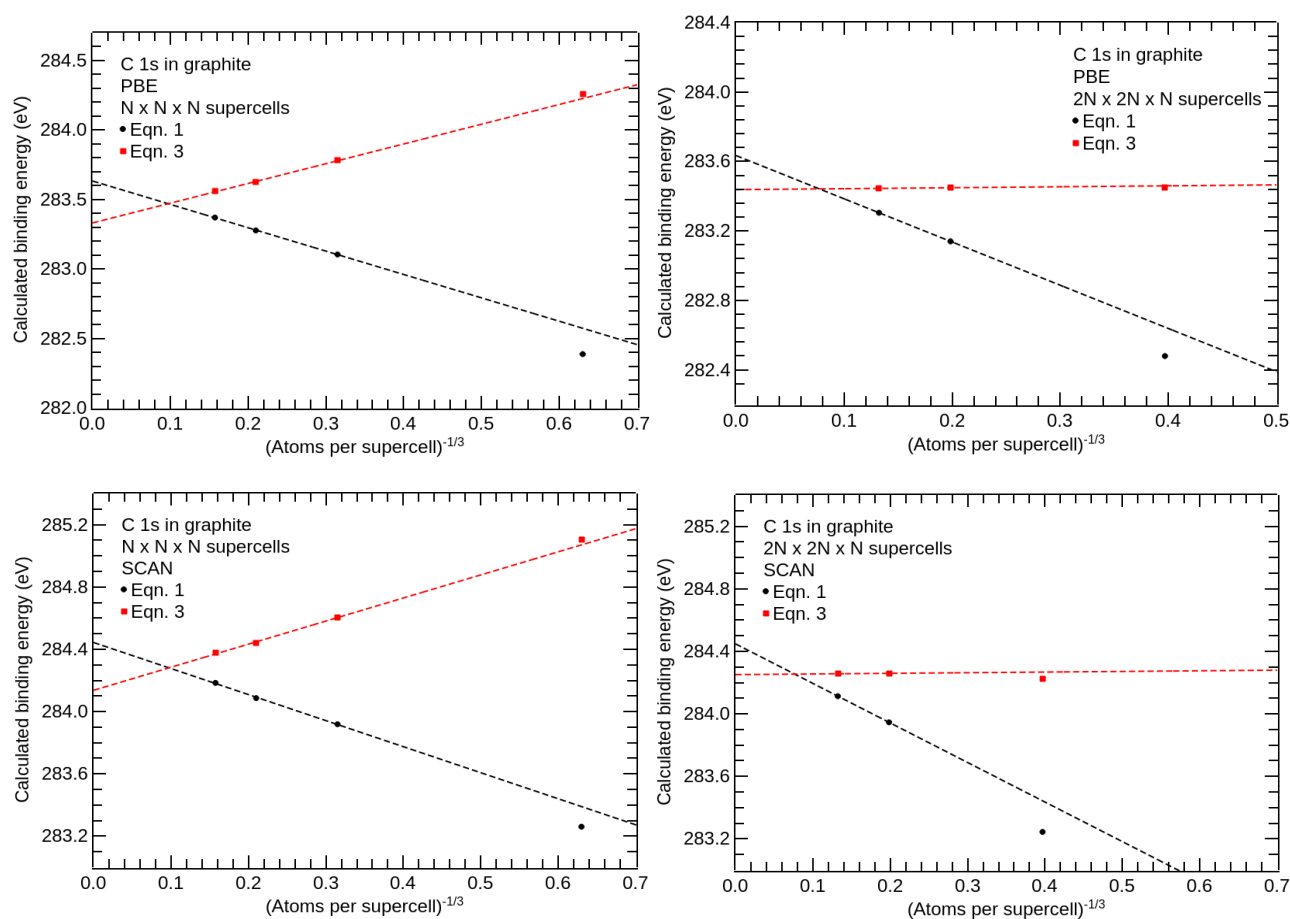

## hex-BN

| Supercell | Atoms per<br>supercell | (Atoms per<br>supercell) <sup>(-1/3)</sup> | B 1s B.E.,<br>Eqn. 1, PBE | B 1s B.E.,<br>Eqn. 3, PBE | N 1s B.E.,<br>Eqn. 1, PBE | N 1s B.E.,<br>Eqn. 3, PBE |
|-----------|------------------------|--------------------------------------------|---------------------------|---------------------------|---------------------------|---------------------------|
| 2x2x1     | 16                     | 0.397                                      | 187.14                    | 187.41                    | 394.93                    | 395.20                    |
| 4x4x2     | 128                    | 0.198                                      | 187.42                    | 187.48                    | 395.34                    | 395.40                    |
| 6x6x3     | 432                    | 0.132                                      | 187.54                    | 187.56                    | 395.48                    | 395.50                    |

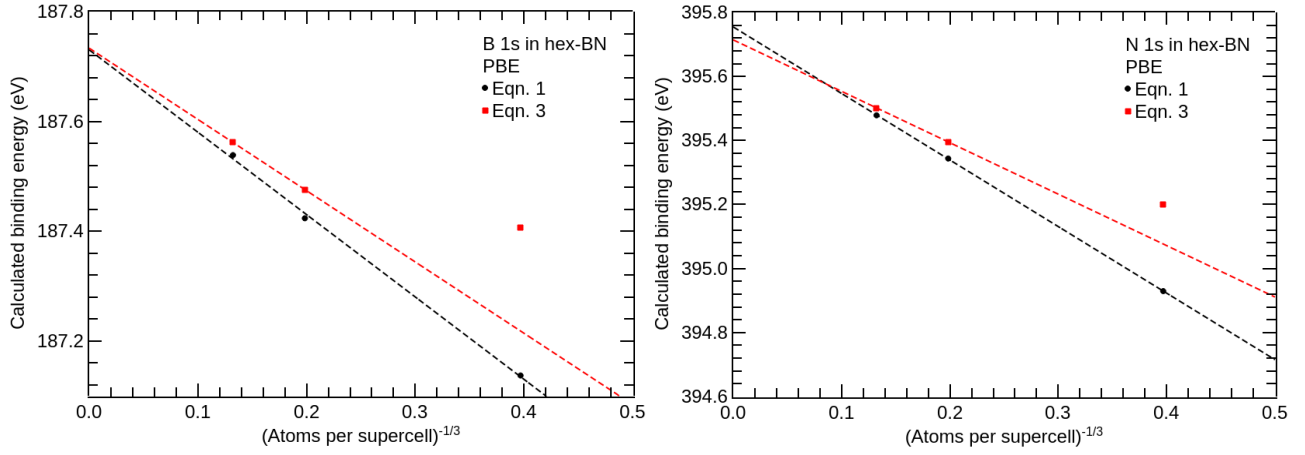

| Supercell | Atoms per<br>supercell | (Atoms per<br>supercell) <sup>(-1/3)</sup> | B 1s B.E.,<br>Eqn. 1, SCAN | B 1s B.E.,<br>Eqn. 3, SCAN | N 1s B.E.,<br>Eqn. 1, SCAN | N 1s B.E.,<br>Eqn. 3, SCAN |
|-----------|------------------------|--------------------------------------------|----------------------------|----------------------------|----------------------------|----------------------------|
| 2x2x1     | 16                     | 0.397                                      | 187.81                     | 188.07                     | 395.54                     | 395.80                     |
| 4x4x2     | 128                    | 0.198                                      | 188.10                     | 188.15                     | 395.96                     | 396.01                     |
| 6x6x3     | 432                    | 0.132                                      | 188.22                     | 188.25                     | 396.11                     | 396.13                     |

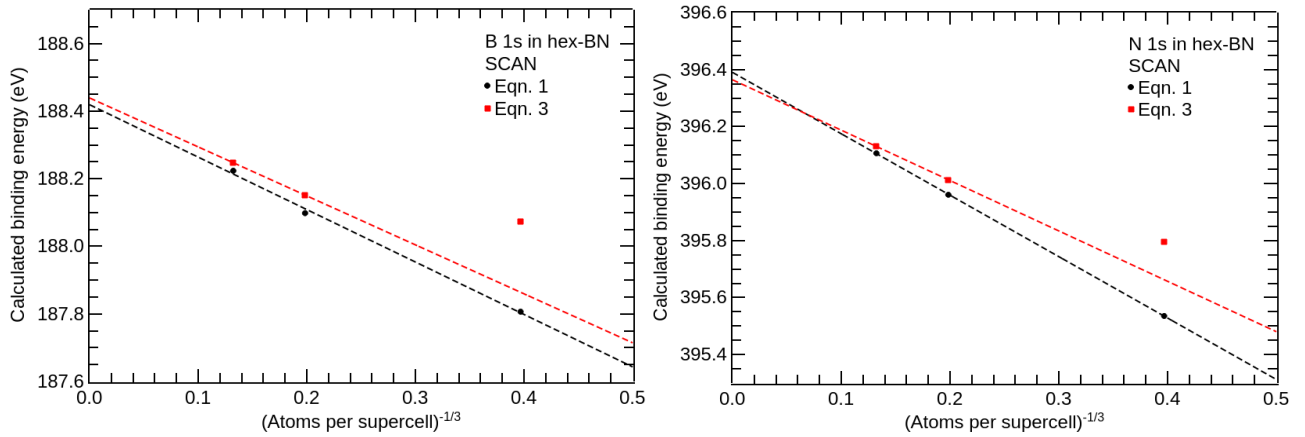

# Lithium

| Supercell | Atoms per<br>supercell | (Atoms per<br>supercell) <sup>(-1/3)</sup> | Li 1s B.E.,<br>Eqn. 1, PBE | Li 1s B.E.,<br>Eqn. 3, PBE | Li 1s B.E.,<br>Eqn. 1, SCAN | Li 1s B.E.,<br>Eqn. 3, SCAN |
|-----------|------------------------|--------------------------------------------|----------------------------|----------------------------|-----------------------------|-----------------------------|
| 1x1x1     | 1                      | 1.000                                      | 54.73                      | 54.83                      | 55.08                       | 55.15                       |
| 2x2x2     | 8                      | 0.500                                      | 54.64                      | 54.65                      | 54.57                       | 54.57                       |
| 3x3x3     | 27                     | 0.333                                      | 54.65                      | 54.64                      | 54.88                       | 54.88                       |
| 4x4x4     | 64                     | 0.250                                      | 54.65                      | 54.64                      | 54.88                       | 54.88                       |
| 5x5x5     | 125                    | 0.200                                      | 54.64                      | 54.64                      | 54.87                       | 54.86                       |

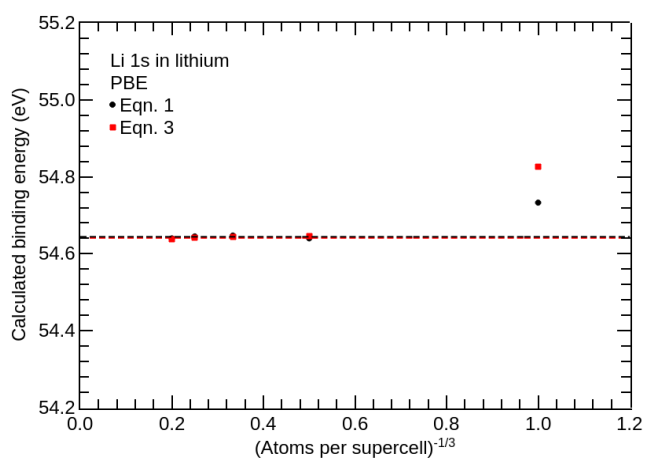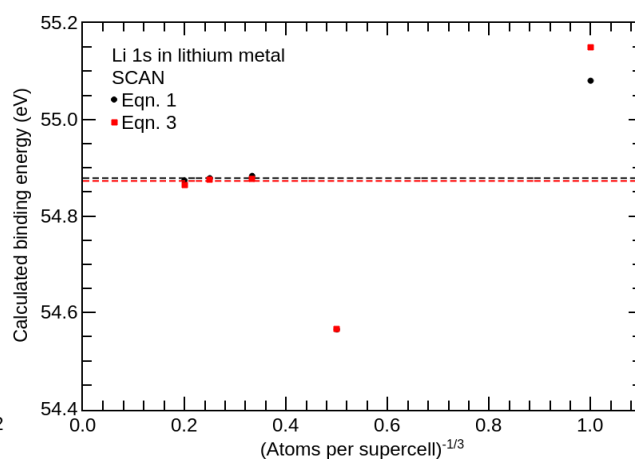

# Magnesium

| Supercell | Atoms per supercell | (Atoms per supercell) <sup>(-1/3)</sup> | Mg 1s B.E.,<br>Eqn. 1, PBE | Mg 1s B.E.,<br>Eqn. 3, PBE | Mg 2p B.E.,<br>Eqn. 1, PBE | Mg 2p B.E.,<br>Eqn. 3, PBE |
|-----------|---------------------|-----------------------------------------|----------------------------|----------------------------|----------------------------|----------------------------|
| 1x1x1     | 2                   | 0.794                                   | 1300.48                    | 1300.83                    | 43.16                      | 43.51                      |
| 2x2x1     | 8                   | 0.500                                   | 1300.75                    | 1300.84                    | 49.26                      | 49.34                      |
| 3x3x2     | 36                  | 0.303                                   | 1300.84                    | 1300.87                    | 49.39                      | 49.41                      |
| 4x4x3     | 96                  | 0.218                                   | 1300.87                    | 1300.88                    | 49.42                      | 49.43                      |
| 5x5x3     | 150                 | 0.188                                   | 1300.87                    | 1300.88                    | 49.42                      | 49.43                      |
| 6x6x4     | 288                 | 0.151                                   | 1300.87                    | 1300.88                    | 49.43                      | 49.44                      |

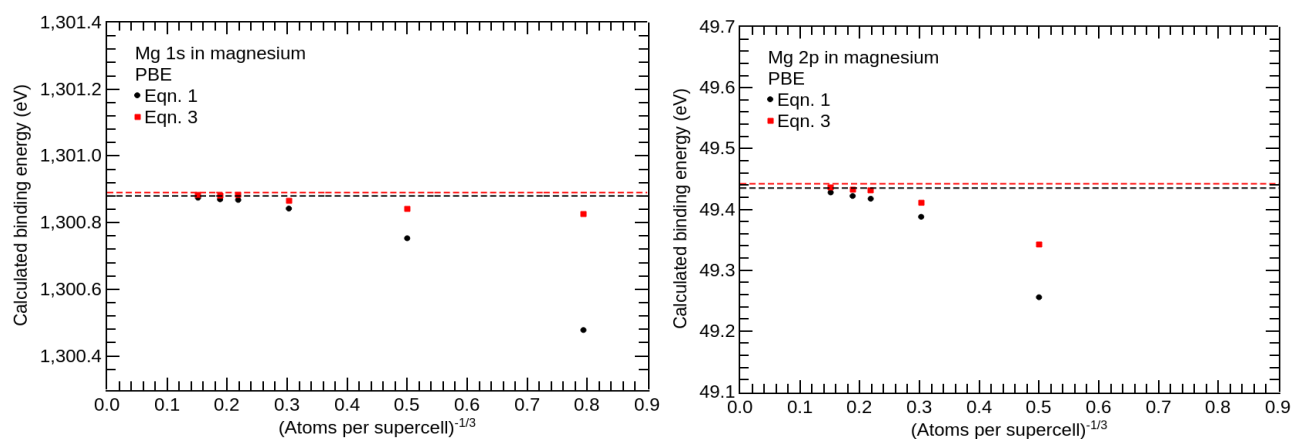

| Supercell | Atoms per supercell | (Atoms per supercell) <sup>(-1/3)</sup> | Mg 1s B.E.,<br>Eqn. 1, SCAN | Mg 1s B.E.,<br>Eqn. 3, SCAN | Mg 2p B.E.,<br>Eqn. 1, SCAN | Mg 2p B.E.,<br>Eqn. 3, SCAN |
|-----------|---------------------|-----------------------------------------|-----------------------------|-----------------------------|-----------------------------|-----------------------------|
| 1x1x1     | 2                   | 0.794                                   | 1302.85                     | 1303.21                     | 50.16                       | 50.52                       |
| 2x2x1     | 8                   | 0.500                                   | 1303.11                     | 1303.20                     | 49.52                       | 49.61                       |
| 3x3x2     | 36                  | 0.303                                   | 1303.22                     | 1303.24                     | 49.63                       | 49.65                       |
| 4x4x3     | 96                  | 0.218                                   | 1303.24                     | 1303.23                     | 49.69                       | 49.68                       |
| 5x5x3     | 150                 | 0.188                                   | 1303.25                     | 1303.26                     | 49.68                       | 49.70                       |
| 6x6x4     | 288                 | 0.151                                   | 1303.25                     | 1303.26                     | 49.70                       | 49.71                       |

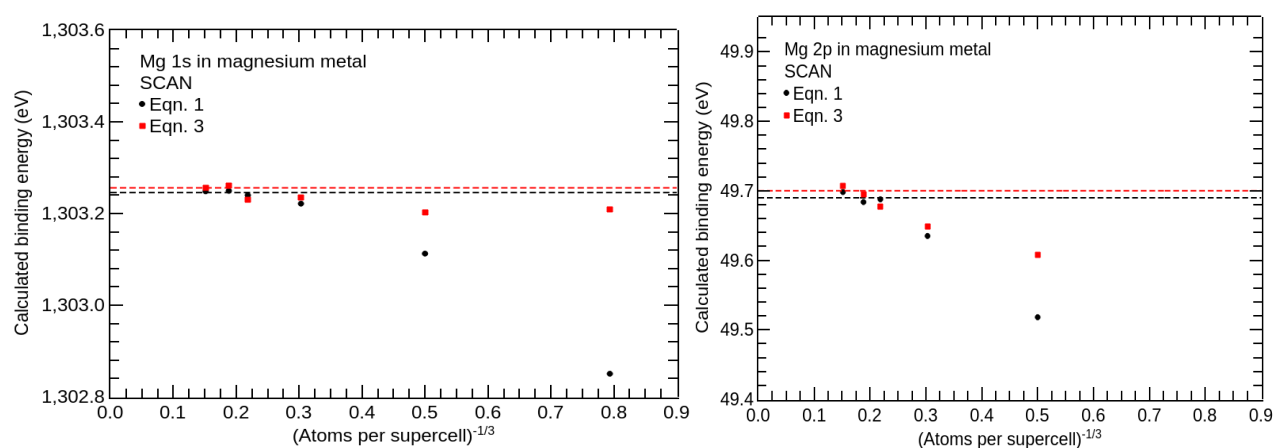

# Silicon

| Supercell | Atoms per<br>supercell | (Atoms per<br>supercell) <sup>-1/3</sup> | Si 2p B.E.,<br>Eqn. 1, PBE | Si 2p B.E.,<br>Eqn. 3, PBE | Si 2p B.E.,<br>Eqn. 1, SCAN | Si 2p B.E.,<br>Eqn. 3, SCAN |
|-----------|------------------------|------------------------------------------|----------------------------|----------------------------|-----------------------------|-----------------------------|
| 1x1x1     | 2                      | 0.794                                    | 97.11                      | 98.22                      | 97.45                       | 98.57                       |
| 2x2x2     | 16                     | 0.397                                    | 98.26                      | 98.64                      | 98.63                       | 99.00                       |
| 3x3x3     | 54                     | 0.265                                    | 98.43                      | 98.61                      | 98.80                       | 98.98                       |
| 4x4x4     | 128                    | 0.198                                    | 98.51                      | 98.61                      | 98.89                       | 98.99                       |
| 5x5x5     | 250                    | 0.159                                    | 98.55                      | 98.62                      | 98.96                       | 99.04                       |

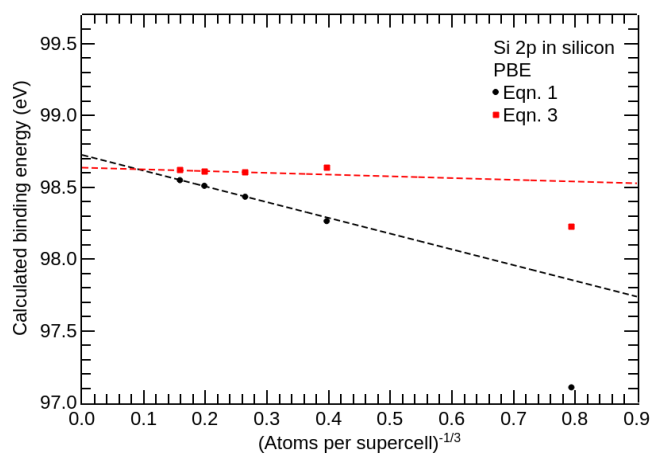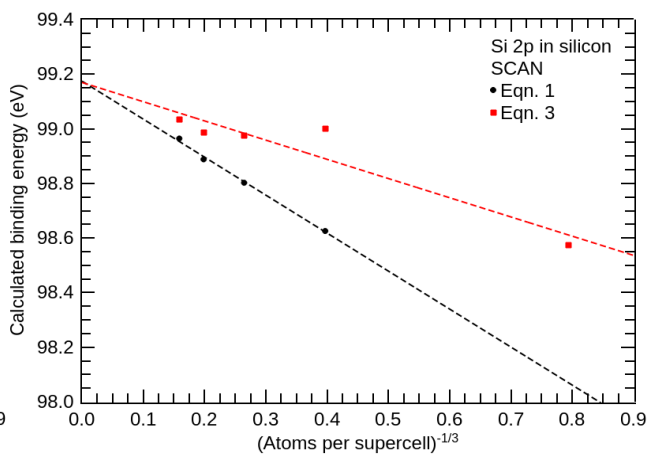

# Sodium

| Supercell | Atoms per supercell | (Atoms per supercell) <sup>(-1/3)</sup> | Na 1s B.E.,<br>Eqn. 1, PBE | Na 1s B.E.,<br>Eqn. 3, PBE | Na 2p B.E.,<br>Eqn. 1, PBE | Na 2p B.E.,<br>Eqn. 3, PBE |
|-----------|---------------------|-----------------------------------------|----------------------------|----------------------------|----------------------------|----------------------------|
| 1x1x1     | 1                   | 1.000                                   | 1069.45                    | 1069.61                    | 30.51                      | 30.67                      |
| 2x2x2     | 8                   | 0.500                                   | 1069.65                    | 1069.67                    | 30.54                      | 30.56                      |
| 3x3x3     | 27                  | 0.333                                   | 1069.67                    | 1069.68                    | 30.57                      | 30.58                      |
| 4x4x4     | 64                  | 0.250                                   | 1069.68                    | 1069.68                    | 30.59                      | 30.59                      |
| 5x5x5     | 125                 | 0.200                                   | 1069.68                    | 1069.68                    | 30.58                      | 30.59                      |

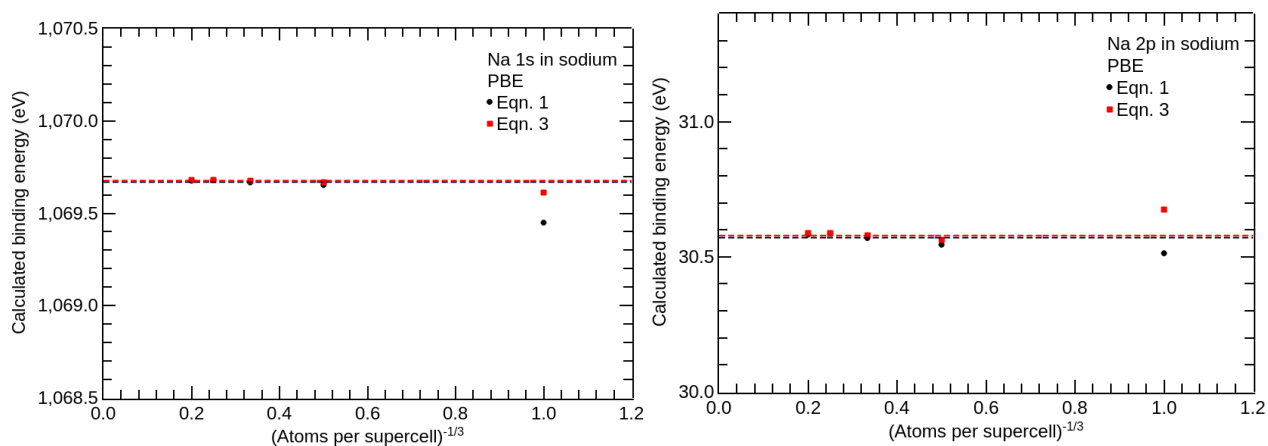

| Supercell | Atoms per supercell | (Atoms per supercell) <sup>(-1/3)</sup> | Na 1s B.E.,<br>Eqn. 1, SCAN | Na 1s B.E.,<br>Eqn. 3, SCAN | Na 2p B.E.,<br>Eqn. 1, SCAN | Na 2p B.E.,<br>Eqn. 3, SCAN |
|-----------|---------------------|-----------------------------------------|-----------------------------|-----------------------------|-----------------------------|-----------------------------|
| 1x1x1     | 1                   | 1.000                                   | 1071.37                     | 1071.51                     | 31.48                       | 31.63                       |
| 2x2x2     | 8                   | 0.500                                   | 1071.55                     | 1071.56                     | 30.63                       | 30.65                       |
| 3x3x3     | 27                  | 0.333                                   | 1071.56                     | 1071.57                     | 30.64                       | 30.65                       |
| 4x4x4     | 64                  | 0.250                                   | 1071.58                     | 1071.58                     | 30.65                       | 30.66                       |
| 5x5x5     | 125                 | 0.200                                   | 1071.57                     | 1071.58                     | 30.65                       | 30.66                       |

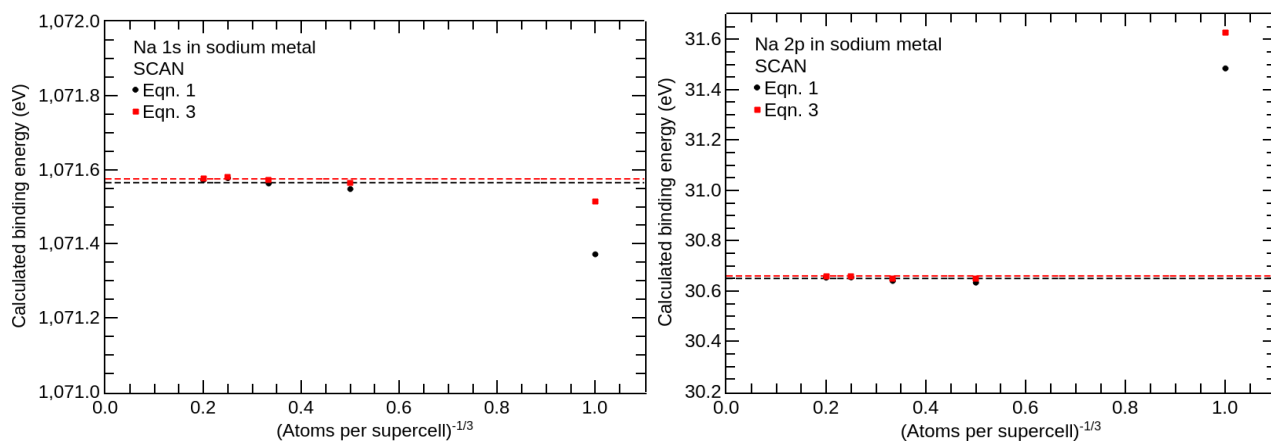

## Numerical verification of Eqn. 2

Plots of the difference between the  $\Delta$ SCF result for the first ionization energy, and the negative Kohn-Sham eigenvalue of the highest occupied state, as a function of the inverse cube root of the number of atoms per supercell, are provided for all materials considered in this work.

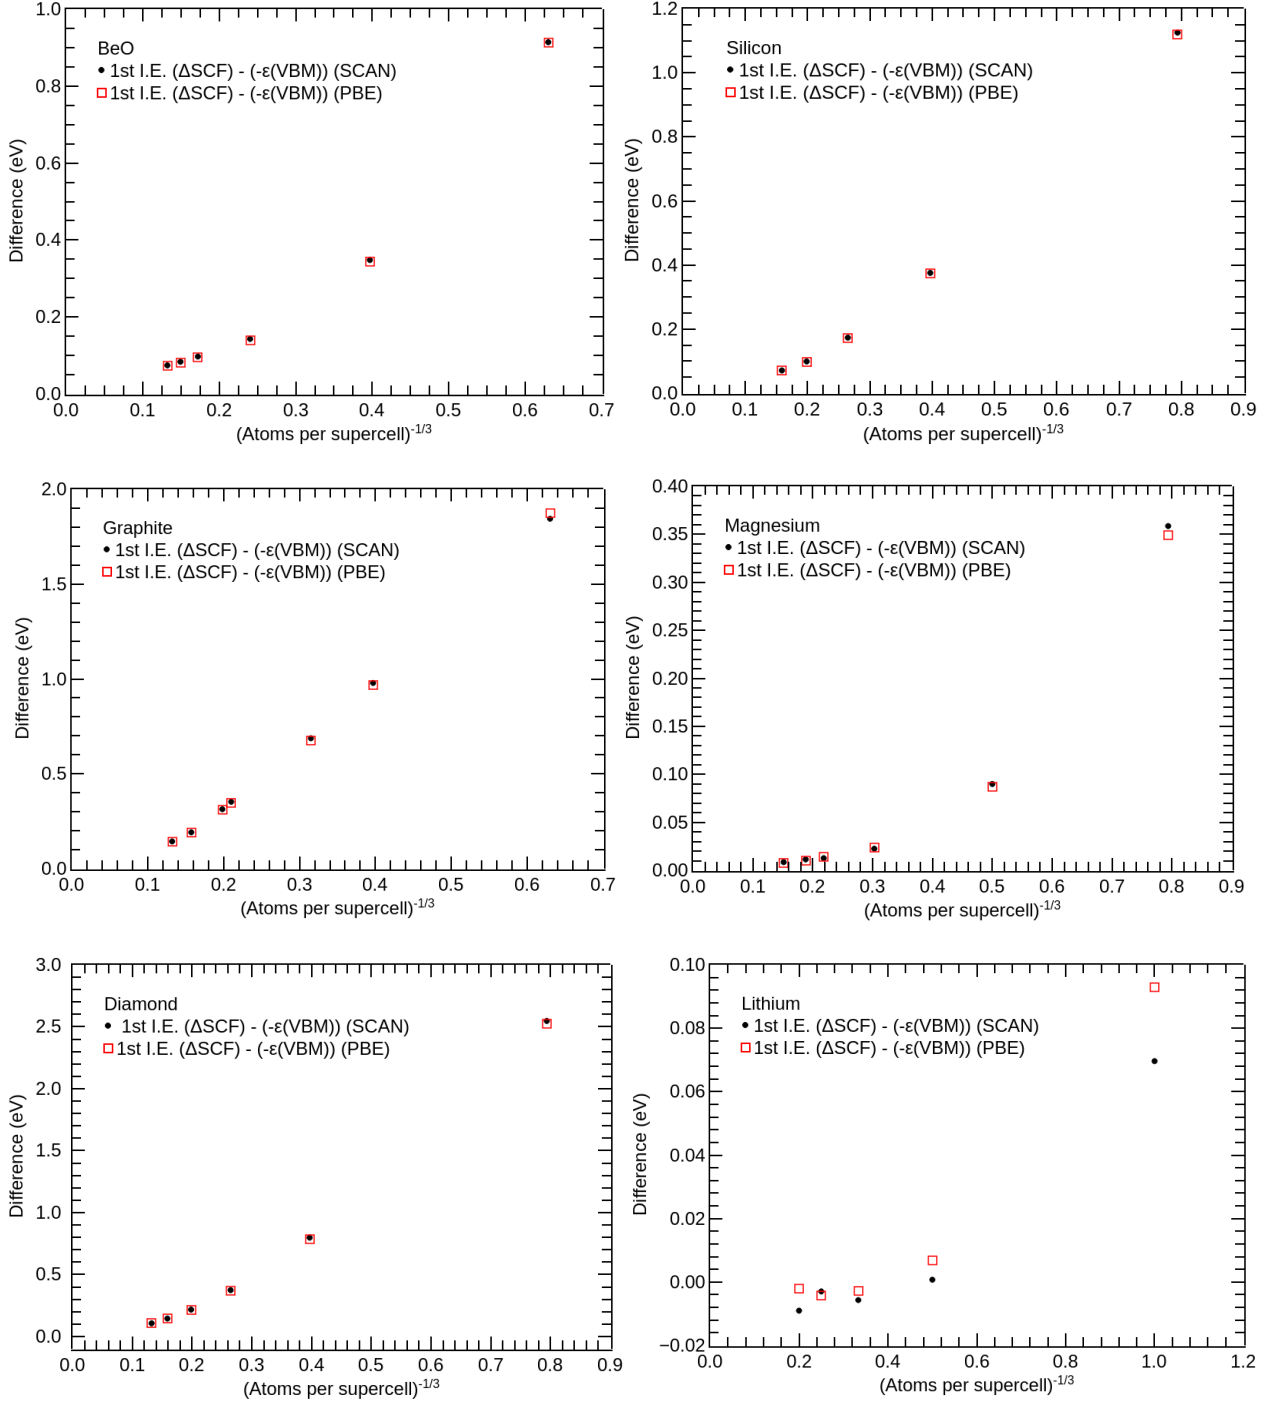

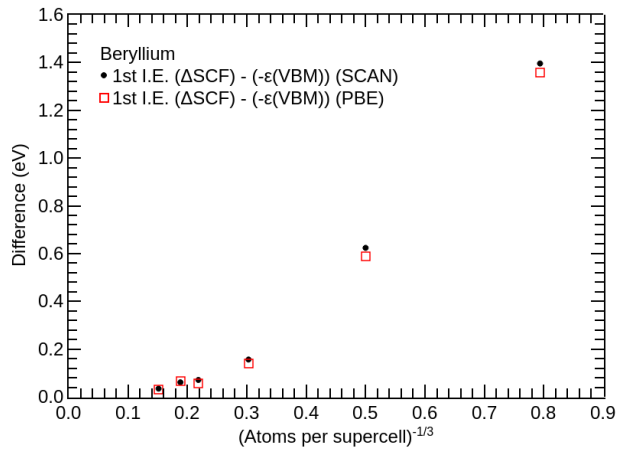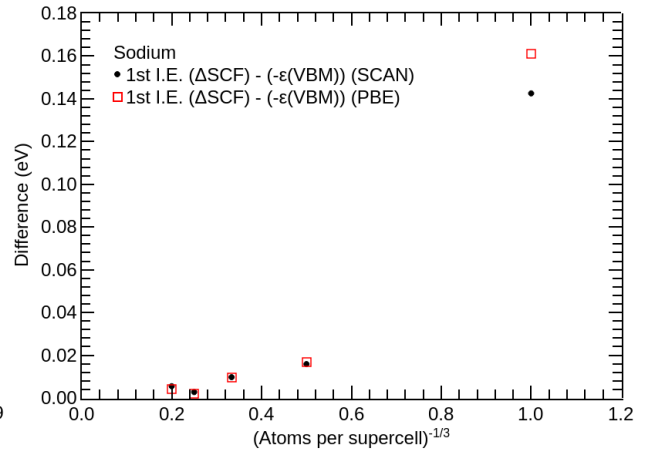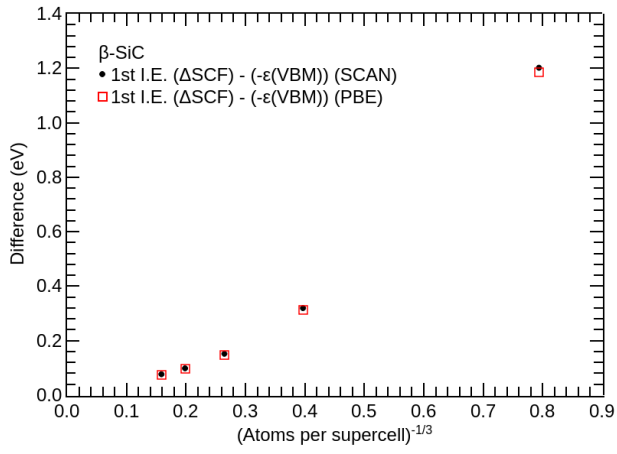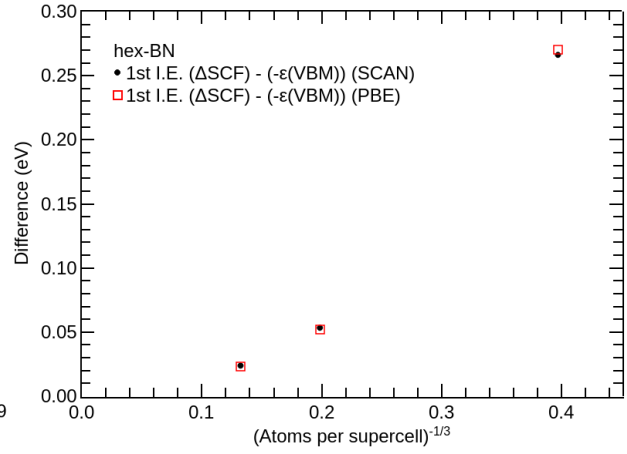

# Structures and k-point grids used in the GW and GW $\Gamma$ calculations

The lattice vectors and the atomic positions are given in units of Ångström.

## BeO

|                |             |              |              |    |
|----------------|-------------|--------------|--------------|----|
| lattice_vector | 1.342104220 | 2.324592698  | 0.000000000  |    |
| lattice_vector | 1.342104220 | -2.324592698 | 0.000000000  |    |
| lattice_vector | 0.000000000 | 0.000000000  | -4.362848360 |    |
| atom           | 1.342104220 | -0.774864233 | 0.000000000  | Be |
| atom           | 1.342104220 | 0.774864233  | -2.181424180 | Be |
| atom           | 1.342104220 | -0.774864233 | -2.711073971 | O  |
| atom           | 1.342104220 | 0.774864233  | -0.529649791 | O  |

k-point grid: (12, 12, 8)

## Be metal

|                |              |             |             |    |
|----------------|--------------|-------------|-------------|----|
| lattice_vector | 2.261367683  | 0.000000000 | 0.000000000 |    |
| lattice_vector | -1.130683842 | 1.958401861 | 0.000000000 |    |
| lattice_vector | 0.000000000  | 0.000000000 | 3.571042160 |    |
| atom           | 0.000000000  | 1.305601241 | 2.678281620 | Be |
| atom           | 1.130683842  | 0.652800620 | 0.892760540 | Be |

k-point grid: (16, 16, 9)

## $\beta$ -SiC

|                |             |             |             |    |
|----------------|-------------|-------------|-------------|----|
| lattice_vector | 2.170890371 | 2.170890371 | 0.000000000 |    |
| lattice_vector | 0.000000000 | 2.170890371 | 2.170890371 |    |
| lattice_vector | 2.170890371 | 0.000000000 | 2.170890371 |    |
| atom           | 0.000000000 | 0.000000000 | 0.000000000 | Si |
| atom           | 1.085445186 | 1.085445186 | 1.085445186 | C  |

k-point grid: (12, 12, 12)

## Diamond

|                |                   |                   |                   |   |
|----------------|-------------------|-------------------|-------------------|---|
| lattice_vector | 2.50306525298690  | 0.000000000000000 | 0.000000000000000 |   |
| lattice_vector | 1.25153262649345  | 2.167718096416780 | 0.000000000000000 |   |
| lattice_vector | 1.25153262649345  | 0.722572698805593 | 2.0437442209028   |   |
| atom           | 0.625766313246725 | 0.361286349402796 | 0.25546802761285  | C |
| atom           | 4.380364192727070 | 2.529004445819570 | 1.78827619328995  | C |

k-point grid: (12, 12, 12)

## Graphite

|                |             |              |                |
|----------------|-------------|--------------|----------------|
| lattice_vector | 1.225034982 | 2.121822829  | 0.000000000    |
| lattice_vector | 1.225034982 | -2.121822829 | 0.000000000    |
| lattice_vector | 0.000000000 | 0.000000000  | -6.909437660   |
| atom           | 0.000000000 | 0.000000000  | -5.182078245 C |
| atom           | 0.000000000 | 0.000000000  | -1.727359415 C |
| atom           | 1.225034982 | -0.707274276 | -5.182078245 C |
| atom           | 1.225034982 | 0.707274276  | -1.727359415 C |

k-point grid: (14, 14, 4)

## hex-BN

|                |              |             |               |
|----------------|--------------|-------------|---------------|
| lattice_vector | 2.494340000  | 0.000000000 | 0.000000000   |
| lattice_vector | -1.247170000 | 2.160161806 | 0.000000000   |
| lattice_vector | 0.000000000  | 0.000000000 | 6.756746360   |
| atom           | 0.000000000  | 0.000000000 | 3.378373180 B |
| atom           | 0.000000000  | 1.440107870 | 0.000000000 B |
| atom           | 0.000000000  | 0.000000000 | 0.000000000 N |
| atom           | 0.000000000  | 1.440107870 | 3.378373180 N |

k-point grid: (14, 14, 5)

## Li metal

|                |             |             |                |
|----------------|-------------|-------------|----------------|
| lattice_vector | 3.481664463 | 0.000000000 | 0.000000000    |
| lattice_vector | 0.000000000 | 3.481664463 | 0.000000000    |
| lattice_vector | 0.000000000 | 0.000000000 | 3.481664463    |
| atom           | 0.000000000 | 0.000000000 | 0.000000000 Li |
| atom           | 1.740832232 | 1.740832232 | 1.740832232 Li |

k-point grid: (14, 14, 14)

## Mg metal

|                |              |             |                |
|----------------|--------------|-------------|----------------|
| lattice_vector | 3.160811260  | 0.000000000 | 0.000000000    |
| lattice_vector | -1.580405630 | 2.737342847 | 0.000000000    |
| lattice_vector | 0.000000000  | 0.000000000 | 5.163388560    |
| atom           | 0.000000000  | 1.824895232 | 1.290847140 Mg |
| atom           | 1.580405630  | 0.912447616 | 3.872541420 Mg |

k-point grid: (14, 14, 8)

## Silicon

|                |             |             |             |    |
|----------------|-------------|-------------|-------------|----|
| lattice_vector | 0.000000000 | 2.716933420 | 2.716933420 |    |
| lattice_vector | 2.716933420 | 0.000000000 | 2.716933420 |    |
| lattice_vector | 2.716933420 | 2.716933420 | 0.000000000 |    |
| atom           | 0.000000000 | 0.000000000 | 0.000000000 | Si |
| atom           | 1.358466710 | 1.358466710 | 1.358466710 | Si |

k-point grid: (12, 12, 12)

## Na metal

|                |             |             |             |    |
|----------------|-------------|-------------|-------------|----|
| lattice_vector | 4.192608683 | 0.000000000 | 0.000000000 |    |
| lattice_vector | 0.000000000 | 4.192608683 | 0.000000000 |    |
| lattice_vector | 0.000000000 | 0.000000000 | 4.192608683 |    |
| atom           | 0.000000000 | 0.000000000 | 0.000000000 | Na |
| atom           | 2.096304342 | 2.096304342 | 2.096304342 | Na |

k-point grid: (12, 12, 12)

# Extrapolation of the GW and GW $\Gamma$ results to $E_{\text{cut}} \Rightarrow +\infty$

## BeO

| $E_{\text{cut}}$ (eV) | $E_{\text{cut}}^{-3/2}$ (eV $^{-3/2}$ ) | nbands | $\epsilon_{\text{max,GW}\Gamma}$ (eV) | $\epsilon_{\text{max,GW}}$ (eV) |
|-----------------------|-----------------------------------------|--------|---------------------------------------|---------------------------------|
| 300                   | 0.0001925                               | 321    | 3.032                                 | 2.898                           |
| 350                   | 0.0001527                               | 404    | 3.029                                 | 2.834                           |
| 400                   | 0.0001250                               | 494    | 3.008                                 | 2.786                           |

Highest occupied state at k-point 0: (0.000, 0.000, 0.000)

$\epsilon_{\text{max,PBE}}$ : 4.85 eV

Extrapolated  $\epsilon_{\text{max,GW}\Gamma\text{@PBE}}$ : 2.97 eV

Extrapolated  $\epsilon_{\text{max,GW@PBE}}$ : 2.58 eV

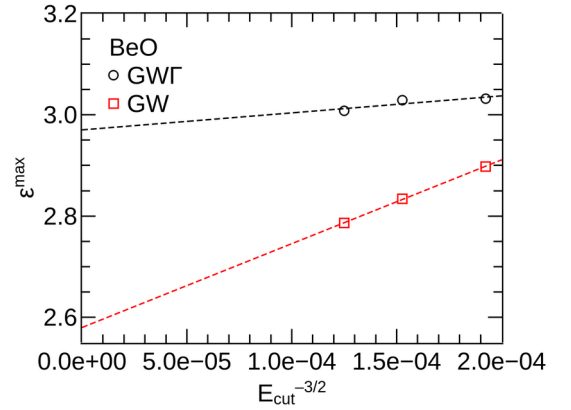

## Be metal

| $E_{\text{cut}}$ (eV) | $E_{\text{cut}}^{-3/2}$ (eV $^{-3/2}$ ) | nbands | $\epsilon_{\text{max,GW}\Gamma}$ (eV) | $\epsilon_{\text{max,GW}}$ (eV) |
|-----------------------|-----------------------------------------|--------|---------------------------------------|---------------------------------|
| 300                   | 0.0001925                               | 186    | 7.93                                  | 7.233                           |
| 350                   | 0.0001527                               | 235    | 7.936                                 | 7.226                           |
| 400                   | 0.0001250                               | 287    | 7.929                                 | 7.222                           |

Highest occupied state at k-point 151: (0.438, -0.125, 0.000)

$\epsilon_{\text{max,PBE}}$ : 7.47 eV

Extrapolated  $\epsilon_{\text{max,GW}\Gamma\text{@PBE}}$ : 7.93 eV

Extrapolated  $\epsilon_{\text{max,GW@PBE}}$ : 7.20 eV

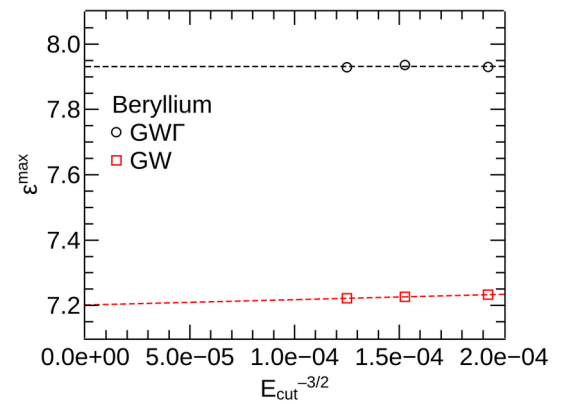

## $\beta$ -SiC

| $E_{\text{cut}}$ (eV) | $E_{\text{cut}}^{-3/2}$ (eV $^{-3/2}$ ) | nbands | $\epsilon_{\text{max,GW}\Gamma}$ (eV) | $\epsilon_{\text{max,GW}}$ (eV) |
|-----------------------|-----------------------------------------|--------|---------------------------------------|---------------------------------|
| 300                   | 0.0001925                               | 241    | 8.068                                 | 7.468                           |
| 350                   | 0.0001527                               | 304    | 8.076                                 | 7.44                            |
| 400                   | 0.0001250                               | 371    | 8.061                                 | 7.422                           |

Highest occupied state at k-point 0: (0.000, 0.000, 0.000)

$\epsilon_{\text{max,PBE}}$ : 8.38 eV

Extrapolated  $\epsilon_{\text{max,GW}\Gamma\text{@PBE}}$ : 8.06 eV

Extrapolated  $\epsilon_{\text{max,GW@PBE}}$ : 7.34 eV

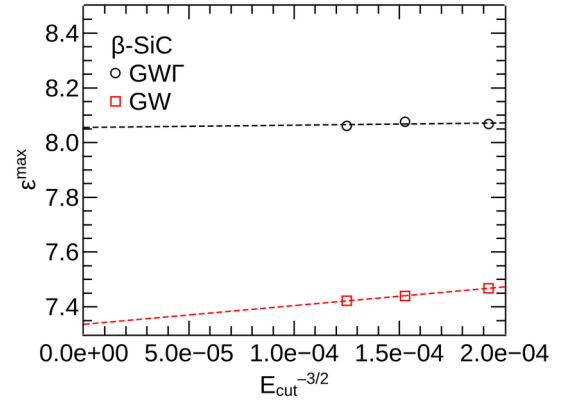

## Diamond

| $E_{\text{cut}}$ (eV) | $E_{\text{cut}}^{-3/2}$ (eV $^{-3/2}$ ) | nbands | $\epsilon_{\text{max,GW}\Gamma}$ (eV) | $\epsilon_{\text{max,GW}}$ (eV) |
|-----------------------|-----------------------------------------|--------|---------------------------------------|---------------------------------|
| 300                   | 0.0001925                               | 130    | 12.038                                | 11.43                           |
| 350                   | 0.0001527                               | 164    | 12.028                                | 11.385                          |
| 400                   | 0.0001250                               | 201    | 12.024                                | 11.355                          |

Highest occupied state at k-point 0: (0.000, 0.000, 0.000)

$\epsilon_{\text{max,PBE}}$ : 12.45 eV

Extrapolated  $\epsilon_{\text{max,GW}\Gamma\text{@PBE}}$ : 12.00 eV

Extrapolated  $\epsilon_{\text{max,GW@PBE}}$ : 11.22 eV

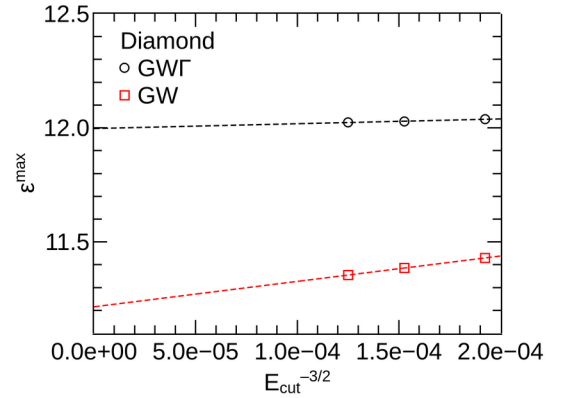

## Graphite

| $E_{\text{cut}}$ (eV) | $E_{\text{cut}}^{-3/2}$ (eV $^{-3/2}$ ) | nbands | $\epsilon_{\text{max,GW}\Gamma}$ (eV) | $\epsilon_{\text{max,GW}}$ (eV) |
|-----------------------|-----------------------------------------|--------|---------------------------------------|---------------------------------|
| 300                   | 0.0001925                               | 423    | 5.898                                 | 5.259                           |
| 350                   | 0.0001527                               | 534    | 5.895                                 | 5.236                           |
| 400                   | 0.0001250                               | 652    | 5.901                                 | 5.221                           |

Highest occupied state at k-point 45: (0.357, 0.357, 0.000)

$\epsilon_{\text{max,PBE}}$ : 5.569 eV

Extrapolated  $\epsilon_{\text{max,GW}\Gamma\text{@PBE}}$ : 5.90 eV

Extrapolated  $\epsilon_{\text{max,GW@PBE}}$ : 5.15 eV

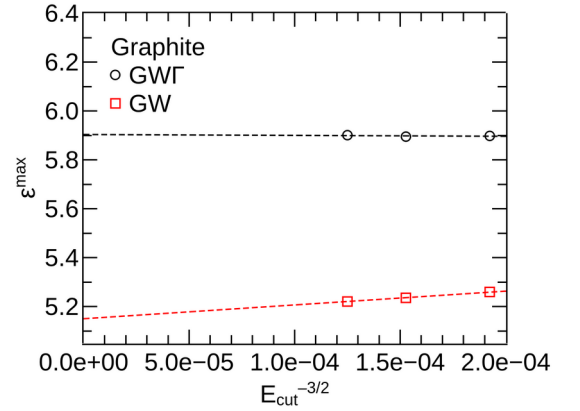

## hex-BN

| $E_{\text{cut}}$ (eV) | $E_{\text{cut}}^{-3/2}$ (eV $^{-3/2}$ ) | nbands | $\epsilon_{\text{max,GW}\Gamma}$ (eV) | $\epsilon_{\text{max,GW}}$ (eV) |
|-----------------------|-----------------------------------------|--------|---------------------------------------|---------------------------------|
| 300                   | 0.0001925                               | 429    | 3.114                                 | 2.695                           |
| 350                   | 0.0001527                               | 541    | 3.105                                 | 2.655                           |
| 400                   | 0.0001250                               | 661    | 3.114                                 | 2.627                           |

Highest occupied state at k-point 36: (0.357, 0.357, 0.000)

$\epsilon_{\text{max,PBE}}$ : 3.95 eV

Extrapolated  $\epsilon_{\text{max,GW}\Gamma\text{@PBE}}$ : 3.11 eV

Extrapolated  $\epsilon_{\text{max,GW@PBE}}$ : 2.50 eV

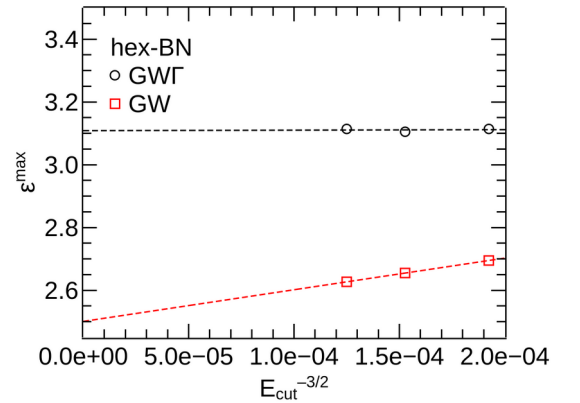

## Li metal

| $E_{\text{cut}}$ (eV) | $E_{\text{cut}}^{-3/2}$ (eV $^{-3/2}$ ) | nbands | $\epsilon_{\text{max,GW}\Gamma}$ (eV) | $\epsilon_{\text{max,GW}}$ (eV) |
|-----------------------|-----------------------------------------|--------|---------------------------------------|---------------------------------|
| 300                   | 0.0001925                               | 497    | 0.288                                 | -0.118                          |
| 350                   | 0.0001527                               | 627    | 0.288                                 | -0.119                          |
| 400                   | 0.0001250                               | 766    | 0.288                                 | -0.119                          |

Highest occupied state at k-point 97: (0.500, 0.286, 0.214)

$\epsilon_{\text{max,PBE}}$ : 0.22 eV

Extrapolated  $\epsilon_{\text{max,GW}\Gamma\text{@PBE}}$ : 0.29 eV

Extrapolated  $\epsilon_{\text{max,GW@PBE}}$ : -0.12 eV

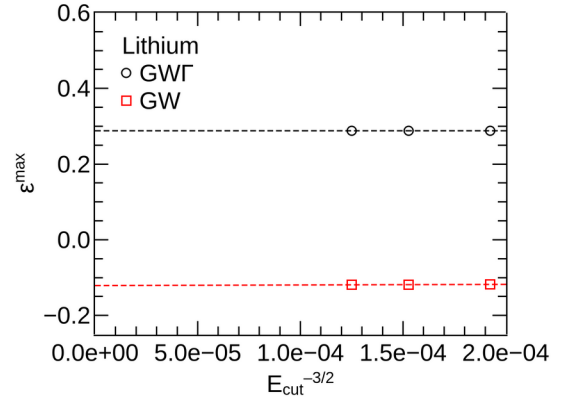

## Mg metal

| $E_{\text{cut}}$ (eV) | $E_{\text{cut}}^{-3/2}$ (eV $^{-3/2}$ ) | nbands | $\epsilon_{\text{max,GW}\Gamma}$ (eV) | $\epsilon_{\text{max,GW}}$ (eV) |
|-----------------------|-----------------------------------------|--------|---------------------------------------|---------------------------------|
| 300                   | 0.0001925                               | 527    | 3.954                                 | 3.3                             |
| 350                   | 0.0001527                               | 664    | 3.947                                 | 3.299                           |
| 400                   | 0.0001250                               | 811    | 3.957                                 | 3.299                           |

Highest occupied state at k-point 66: (0.357, -0.143, 0.000)

$\epsilon_{\text{max,PBE}}$ : 3.75 eV

Extrapolated  $\epsilon_{\text{max,GW}\Gamma\text{@PBE}}$ : 3.96 eV

Extrapolated  $\epsilon_{\text{max,GW@PBE}}$ : 3.30 eV

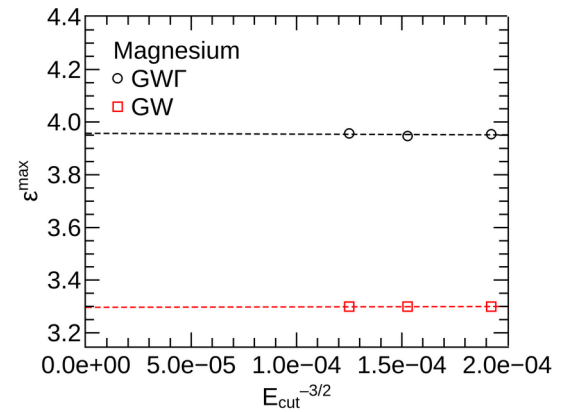

## Silicon

| $E_{\text{cut}}$ (eV) | $E_{\text{cut}}^{-3/2}$ (eV $^{-3/2}$ ) | nbands | $\epsilon_{\text{max,GW}\Gamma}$ (eV) | $\epsilon_{\text{max,GW}}$ (eV) |
|-----------------------|-----------------------------------------|--------|---------------------------------------|---------------------------------|
| 300                   | 0.0001925                               | 473    | 5.301                                 | 4.652                           |
| 350                   | 0.0001527                               | 596    | 5.307                                 | 4.642                           |
| 400                   | 0.0001250                               | 728    | 5.303                                 | 4.634                           |

Highest occupied state at k-point 0: (0.000, 0.000, 0.000)

$\epsilon_{\text{max,PBE}}$ : 5.30 eV

Extrapolated  $\epsilon_{\text{max,GW}\Gamma\text{@PBE}}$ : 5.31 eV

Extrapolated  $\epsilon_{\text{max,GW@PBE}}$ : 4.60 eV

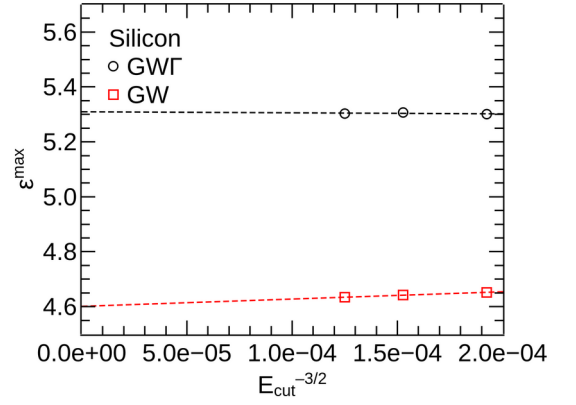

## Na metal

| $E_{\text{cut}}$ (eV) | $E_{\text{cut}}^{-3/2}$ (eV $^{-3/2}$ ) | nbands | $\epsilon_{\text{max,GW}\Gamma}$ (eV) | $\epsilon_{\text{max,GW}}$ (eV) |
|-----------------------|-----------------------------------------|--------|---------------------------------------|---------------------------------|
| 300                   | 0.0001925                               | 869    | 0.326                                 | -0.088                          |
| 350                   | 0.0001527                               | 1095   | 0.326                                 | -0.088                          |
| 400                   | 0.0001250                               | 1338   | 0.327                                 | -0.088                          |

Highest occupied state at k-point 39: (0.417, 0.167, 0.083)

$\epsilon_{\text{max,PBE}}$ : 0.22 eV

Extrapolated  $\epsilon_{\text{max,GW}\Gamma\text{@PBE}}$ : 0.33 eV

Extrapolated  $\epsilon_{\text{max,GW@PBE}}$ : -0.09 eV

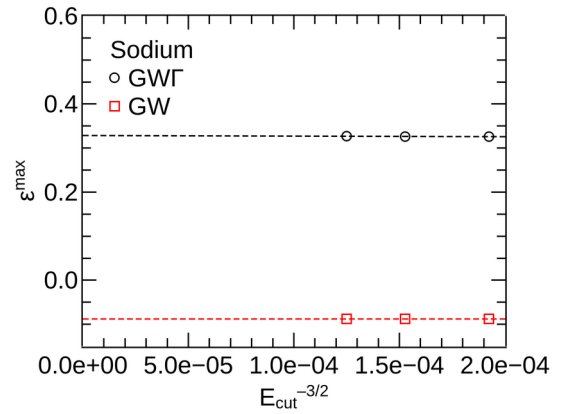

Supplement: Supplementary file 1 [file Supplementary_information.pdf]
